# Supplementary material for: Towards Feasible Counterfactual Explanations: A Taxonomy Guided Template-based NLG Method
Source: arXiv:2310.02019 source file (2023-10-03)
Supplement: Supplementary file 1 [file ap-additional-content.tex]

\section*{Supplementary Material}

Sample responses from participants of user study 2 who viewed explanations generated with (\nxai) and without (\basexai) feature actionability knowledge. Also, All the code for the proposed method, along with the necessary documentation, is available in our online code repository\footnote{https://anonymous.4open.science/r/NLGXAI-0BC6/src/inference.py}.

\begin{table}
\centering
\scalebox{0.78}{
\begin{tabular}{lll}
\hline
Dataset & Explanation with \nxai & Explanation with \basexai \\ \hline
Heart Disease & \begin{tabular}[c]{@{}l@{}}In order to prevent heart problems you would need to change 5 attributes.\\ You would not have heart disease if you,\\ 1), take steps to reduce resting blood pressure to 94.0 and,\\ 2), decrease serum cholesterol from 471.0 to 248.0.\\ 3), raise thalach from 122 to 132.0.\\ 4), increase old peak from 1.0 to 2.0.\\ 5), raise ca from 0 to 1.0.\\ Furthermore, Your age has contributed to having a heart problem.\\ Moreover, sex Male has a higher chance to have a healthy heart compared to\\ sex Female and, stay safe!\end{tabular} & \begin{tabular}[c]{@{}l@{}}In order to prevent heart problems you would need to change 7 attributes.\\ You would not get heart problems if you,\\
1), decrease age to 33.0 and,\\ 2), change sex to Male and,\\3), raise resting blood pressure to 108.0 and,\\ 4), increase chol to 525.0 and, \\ 5), lower thalach to 75.0 and,\\ 6), reduce old peak to 0.0 and, \\7), reduce thal to 0.0. Take care!\end{tabular} \\ \hline
Credit Risk & \begin{tabular}[c]{@{}l@{}}To reduce your credit risk, you would need to change the following 4 attributes.\\ 1), take steps to raise Annual Income to 12000.0 and, \\ 2), take steps to modify Home ownership to RENT and, \\ 3), raise Loan amount to 1600.0. \\ 4), decrease Interest rate to 10.59. \\ In addition, individuals with Employment length 3.0 has a higher chance to have\\ a risk free credit compared to individuals with Employment length 5.0. \\ Wishing you a successful financial journey where your credit remains protected!\end{tabular} & \begin{tabular}[c]{@{}l@{}}To reduce your credit risk, you would need to change the following 5 attributes.\\ 1), raise Annual Income to 12000.0 and,\\ 2), modify Home ownership to RENT and, \\ 3), raise Loan amount to 1600.0 and, \\4), decrease Interest rate to 10.59 and, \\5), decrease Employment length to 3.0.\\ Wishing you a successful financial journey where your credit remains protected!\end{tabular} \\ \hline
Student Performance & \begin{tabular}[c]{@{}l@{}}In order to get a total score that is above the average, you would need to \\ change the following 3 attributes.\\ 1), increase math score to 68.0. \\ 2), raise reading score to 72.0. \\ 3), increase writing score to 64.0. \\ Furthermore,  parental level of education is a contributing factor to the risk\\  of obtaining an overall score of below the average. Good luck with your results!\end{tabular} & \begin{tabular}[c]{@{}l@{}}In order to get a total score that is above the average, you would need to change\\ the following 4 attributes.\\1), increase math score to 68.0 and, \\2), raise reading score to 72.0 and, \\3), increase writing score to 64.0 and,\\ 4), change your parental level of education to bachelor's degree. Good luck with your results!\end{tabular} \\ \hline
\end{tabular}
}
\caption{A sample of responses for \nxai and \basexai.}
\label{tab:userstudy2}
\end{table}

In our second user study, we asked participants a series of questions addressing four criteria: articulation, acceptability, feasibility, and sensitivity. These questions appear in Table \ref{tab:us2Qs}. Additionally, we also asked them to explain their reasons for their choices in an open-ended question.
\begin{table}
\centering
\begin{tabular}{ll}
\hline
\textit{Criteria} & \textit{Questions} \\ \hline
Articulation & \begin{tabular}[c]{@{}l@{}}On a scale of 1 to 5, with 1 being "strongly disagree" and 5 being "strongly agree", \\ how would you rate the statement: "Regardless of accuracy, this explanation is well articulated"?\end{tabular} \\ \hline
Acceptability & \begin{tabular}[c]{@{}l@{}}On a scale of 1 to 5, with 1 being "not at all acceptable" and 5 being "completely acceptable", \\ how would you rate the acceptability of the counterfactual explanation provided to the user?\end{tabular} \\ \hline
Feasiblity & \begin{tabular}[c]{@{}l@{}}On a scale of 1 to 5, with 1 being "not at all feasible" and 5 being "completely feasible", \\ how would you rate the feasibility of the counterfactual explanation provided to the user?\end{tabular} \\ \hline
Sensitivity & \begin{tabular}[c]{@{}l@{}}On a scale of 1 to 5, with 1 being "strongly disagree" and 5 being "strongly agree", \\ to what extent do you believe that sensitive personal characteristics and ethical considerations\\  are appropriately addressed in the counterfactual explanation provided?\end{tabular} \\ \hline
\end{tabular}
\caption{Questions related to 4 criteria of evaluating \nxai}
\label{tab:us2Qs}
\end{table}
